# Supplementary material for: Robust and Precision Satellite Formation Flying Guidance Using Adaptive Optimal Control Techniques
Source: arXiv:2006.01813 source file (2020-05-31)
Supplement: Supplementary file 1 [file Appendix.tex]

\chapter{Appendix} \label{Appendix}
\section{Appendix A}

This Appendix presents the elements of transformation matrix $\Sigma (t)^{-1}$
